# Supplementary material for: Federated pretraining and fine tuning of BERT using clinical notes from multiple silos
Source: arXiv:2002.08562 source file (2020-02-20)
Supplement: Supplementary file 1 [file Appendix.tex]

\appendix

\section{Appendices}
\label{sec:appendix}

\begin{figure*}[t]
  \centering 
  \includegraphics[width=4in]{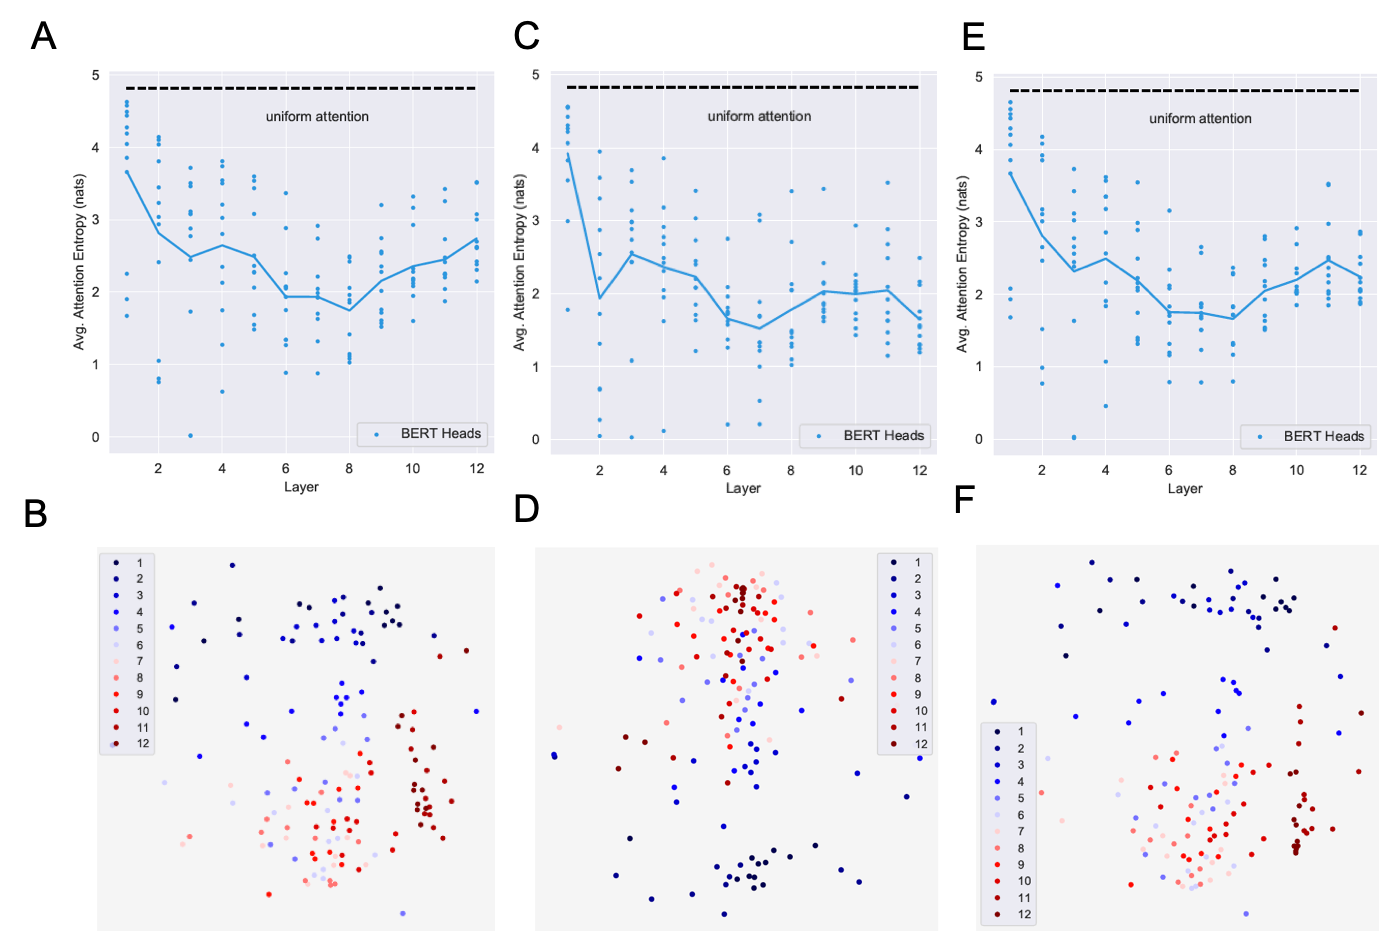} 
  \caption{Appendix figure: Analysis of attention heads  (A,C,E)Entropy of attention heads in different layers in BERTbase, Clinical BERT and federated clinical BERT models.(B,D,F)BERT attention head projects onto two dimentional space}
  \label{fig:Attention_analysis} 
\end{figure*}
